# Supplementary material for: Electronic coupling between Bi nanolines and the Si(001) substrate: An experimental and theoretical study
Source: arXiv:1710.09592 source file (2017-12-05)
Supplement: Supplementary file 1 [file Supplemental_Material.pdf]

# Electronic coupling between Bi nanolines and the Si(001) substrate: An experimental and theoretical study. Supplemental Material

M. Longobardi,[1] C. J. Kirkham,[2,3] R. Villarreal,[1] S. A. Köster,[1] D. R. Bowler,[3,4] and Ch. Renner[1]

[1]*Department of Quantum Matter Physics, University of Geneva, 24 Quai Ernest-Ansermet, CH-1211 Geneva 4, Switzerland*
[2]*National Institute for Materials Science (NIMS), Namiki 1-1, Tsukuba, Ibaraki, 305-0044, Japan*
[3]*London Centre for Nanotechnology and Department of Physics and Astronomy, University College London, London WC1E 6BT, United Kingdom*
[4]*International Center for Materials Nanoarchitectonics (MANA), National Institute for Materials Science (NIMS), Namiki 1-1, Tsukuba, Ibaraki, 305-0044, Japan*

## S1. HIGH BIAS SCANNING TUNNELING MICROSCOPY FEATURES

Here we discuss the STM appearance of the Bi nanolines in the high bias regime, aided by DFT simulations.

### A. Negative bias STM

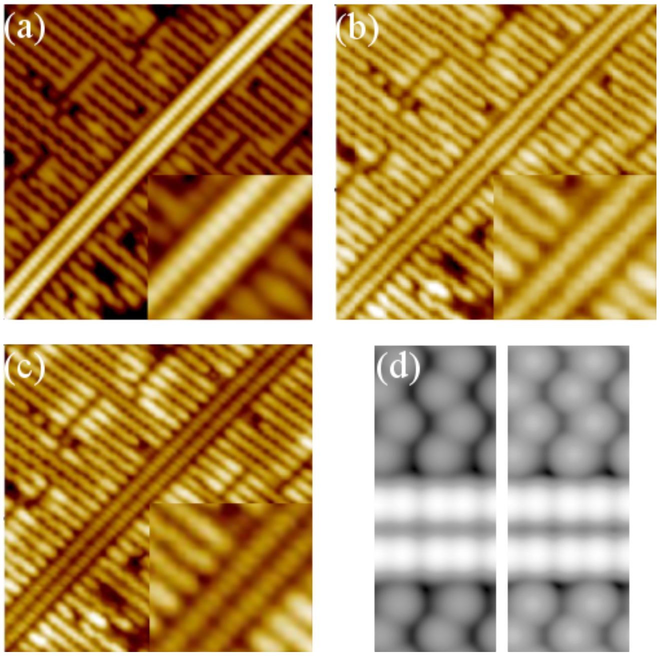


FIG. S1. (Color online) $7.5\times7.6$ nm$^2$ STM micrographs of the same Bi nanoline at (a) $-3.3$ V (0.4 nA), (b) $-3.0$ V (1 nA) and (c) $-2.7$ V (1 nA). Inset shows a $2.0\times1.8$ nm$^2$ magnification of the nanoline. (d) DFT simulated STM micrograph of the Bi nanoline at -3.0 V (left) and -1.0 V (right).

At negative bias, as shown in Fig. S1, the Bi dimers of the nanoline can be imaged as two bright spots corresponding to individual Bi atoms, which we attribute to the $\pi^*$ states. As the bias of the system is lowered, the brightness contrast between the Bi nanolines and the Si background alters, with the nanolines brighter than the background below $-3.0$ V, and dimmer above $-3.0$ V. The lower current used for the -3.3 V image does not affect this conclusion. As the nanolines become dimmer, the bright spots become better defined. The brightness inversion is known as the "antiwire property" of Bi nanolines [1], and can be explained by a semiconductor–like behavior of the Bi nanolines, with a band gap larger than bare Si. Simulations, as shown in (d), reproduce the appearance of the nanoline very well, with bright spots corresponding to Bi atoms in the nanoline and to up Si atoms in the background. The weakening of the Bi nanoline brightness with reducing bias is also reproduced, however not the contrast inversion seen in experiment.

### B. Positive bias STM

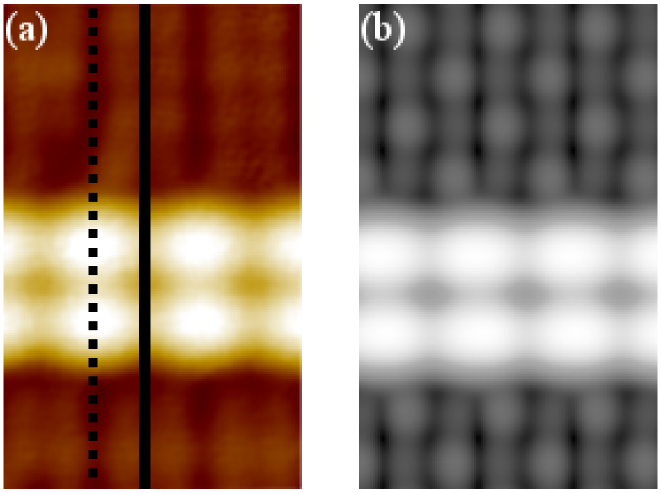


FIG. S2. (Color online) (a) $1.8\times2.9$ nm$^2$ STM micrograph of a Bi nanoline at 2.0 V (0.1 nA).The dashed and solid lines indicate the dimer row centre and trench, respectively. (b) Corresponding DFT simulation at 1.5 V.

Above 1.5 V tunneling bias, the Bi nanoline appears as a double row of elliptical bright spots, as shown in Fig. S2(a), one for every Bi dimer. To assign these ellipses within the Bi nanoline, we rely on the atomically resolved surrounding Si surface. The latter shows stripes of atom pairs separated by dark lines running perpendic-

ular to the Bi nanolines. Naively, one would identify the stripes with the Si dimer rows. However, the STM imaging contrast of the Si(001) surface undergoes a phase shift around 1.35 V [2] due to mixed and backbond electronic states of Si [3]. Therefore, the correct interpretation of the background contrast is that the dark lines correspond to the centre of the Si(001) dimer rows. Therefore, the bright ellipses in Fig. S2(a) correspond to the Bi dimers forming the Bi nanoline. This analysis is verified by the DFT simulation in Fig. S2(b), where the ellipses overlap with the Bi dimer positions.

## S2. INTERMEDIATE BIAS STM

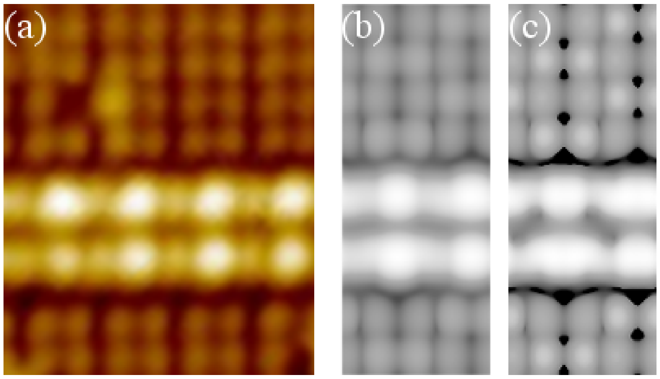


FIG. S3. (Color online) (a) $2.6 \times 3.1$ nm$^2$ experimental STM micrograph of a Bi nanoline at 1.5 V (1 nA), compared against simulated STM for a Bi nanoline on $c(4 \times 2)$ Si at (b) 1.1 V with the $\Gamma$ $k$-point, and (c) 1.0 V without.

In Fig. S3 we demonstrate the importance of including the $\Gamma$ $k$-point for simulations in the intermediate bias regime. As noted in the main text, there is excellent agreement with experiment when the $\Gamma$ $k$-point is included, with both the phase shift of the Bi nanoline and the relative brightness of the two spots reproduced well [Fig. S3(b)]. However, if the $\Gamma$ point is not included, the relative brightness of the two spots is wrong [Fig. S3(c)].

## S3. MODEL OF OVERLAPPING P-ORBITALS

We built a simple analytical model of overlapping $p$-orbitals, based on the structural parameters of the Bi nanoline. A two dimer long section of the Bi nanoline was represented by eight $p$-orbitals, with the relative distances between them matched to experiment. With dimer spacing 1.5 times the dimer length, and row spacing twice the dimer length. The extent of the $p$-orbitals was determined empirically to reproduce the overlaps seen in DFT simulations. The relative orbital phase of the $p$-orbitals, as represented in blue or red, was then arranged to form various bonding (overlapping in phase) or anti-bonding (overlapping out of phase) orbitals, as shown in Fig. S4. The arrangement with anti-bonding orbitals on the Bi dimers and bonding orbitals between them, as shown in (b), closely matches the DFT results.

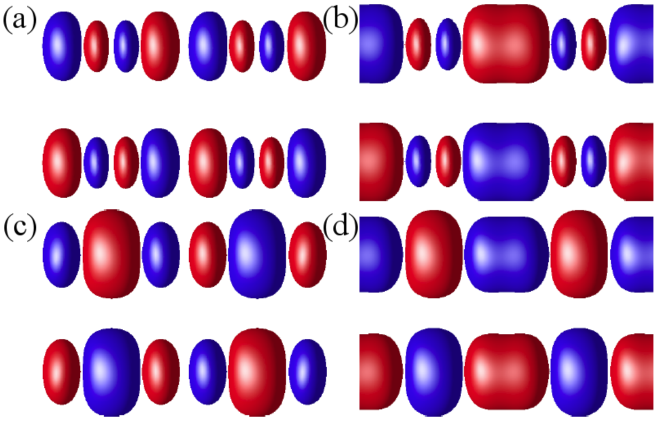


FIG. S4. (Color Online) Model of overlapping $p$-orbitals equivalent to a two dimer long section of the Bi nanoline, with their relative orbital phase represented in blue or red. (a) Anti-bonding in the dimer and trench regions. (b) Anti-bonding in the dimer region and bonding in the trench region. (c) Bonding in the dimer region and anti-bonding in the trench region. (d) Bonding in the dimer and trench regions.

[1] R. H. Miwa, J. M. MacLeod, A. B. McLean, and G. P. Srivastava, Nanotechnology **16**, 2427 (2005).
[2] K. Hata, S. Yasuda, and H. Shigekawa, Phys. Rev. B **60**, 8164 (1999).
[3] H. Okada, Y. Fujimoto, K. Endo, K. Hirose, and Y. Mori, Phys. Rev. B **63**, 195324 (2001).
